# Supplementary material for: SAC: Semantic Attention Composition for Text-Conditioned Image Retrieval
Source: arXiv:2009.01485 source file (2021-10-19)

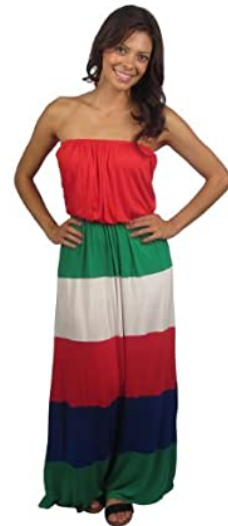

*Has thin straps  
and different  
pattern and more  
autumn colored  
and longer*

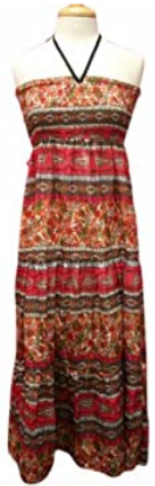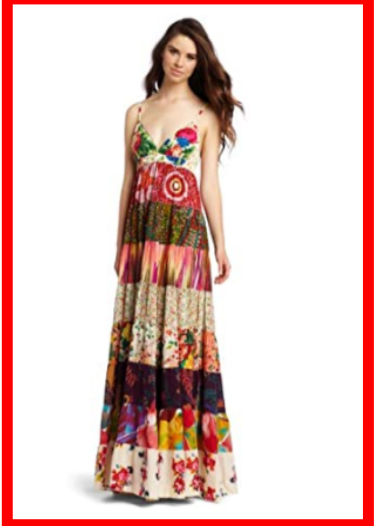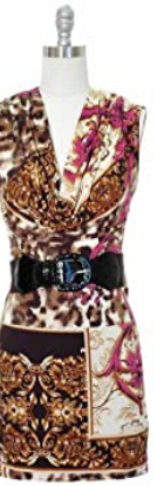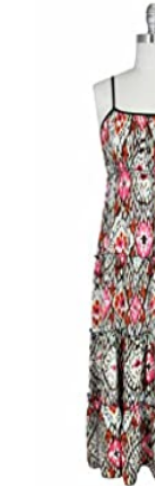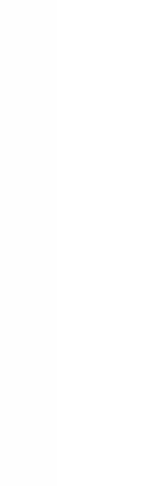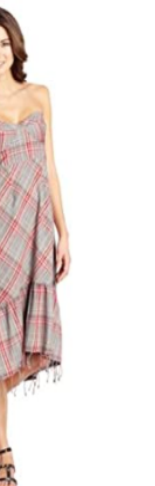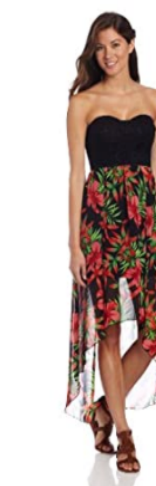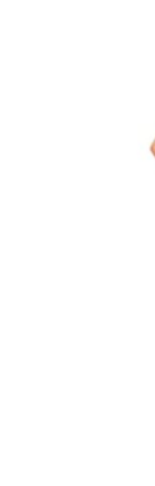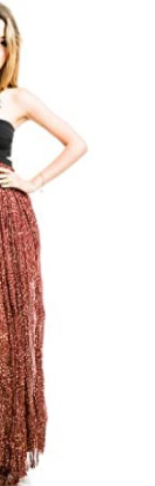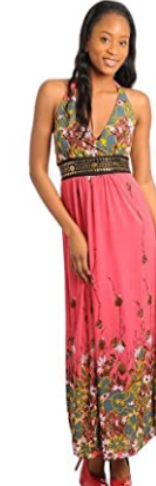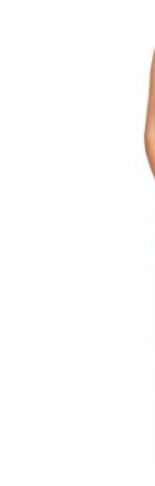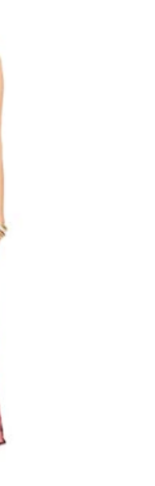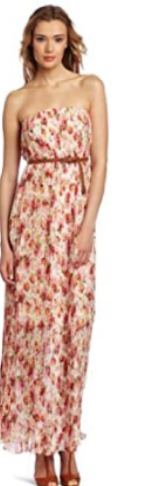

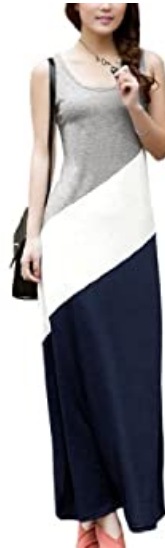

*has a darker long skirt and lighter top. and is gray and fitted at waist*

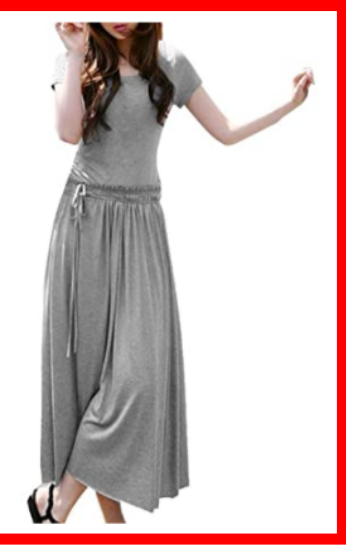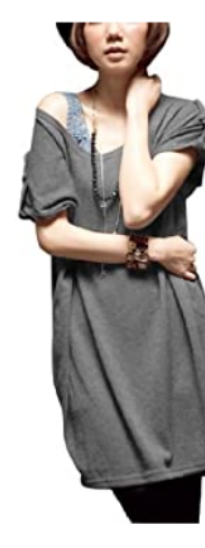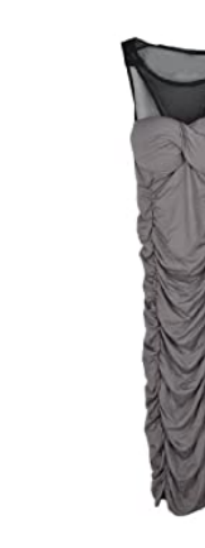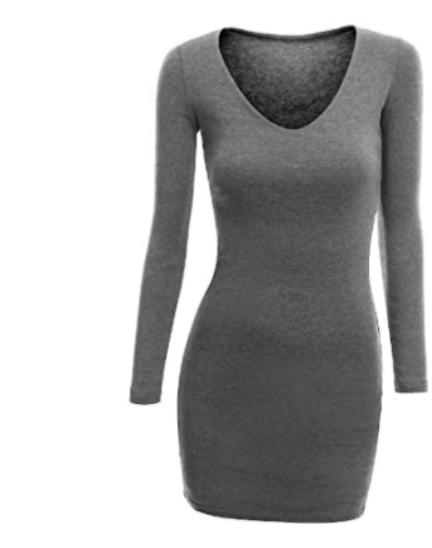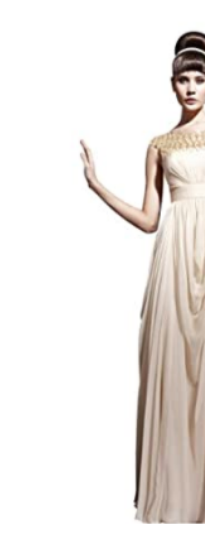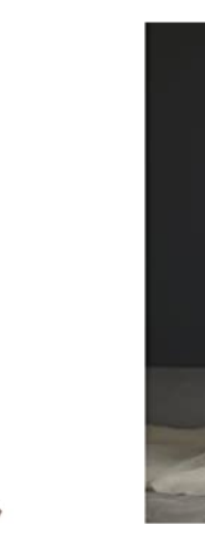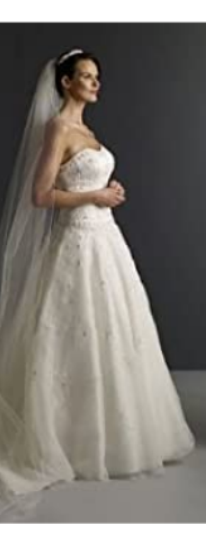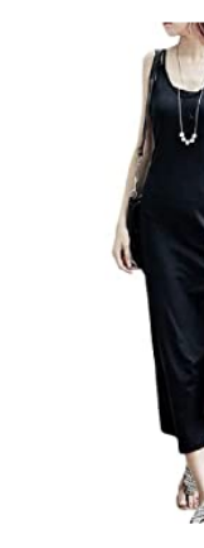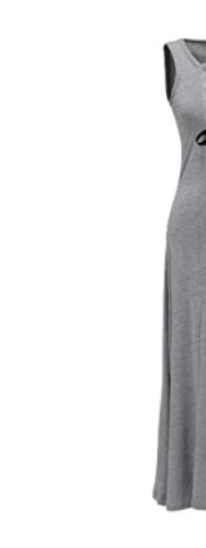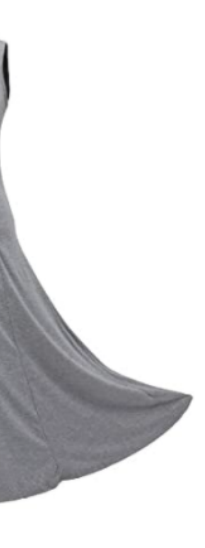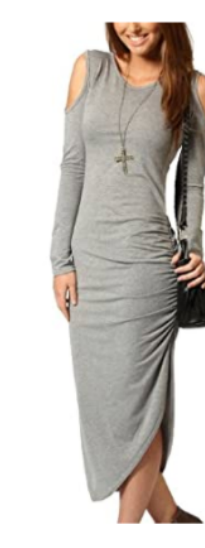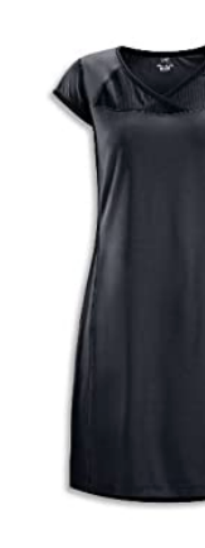

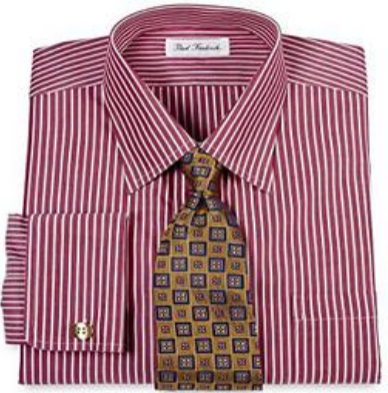

*is green plaid  
and is black  
and grey  
checked with  
a navy tie*

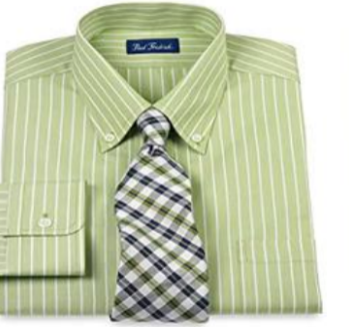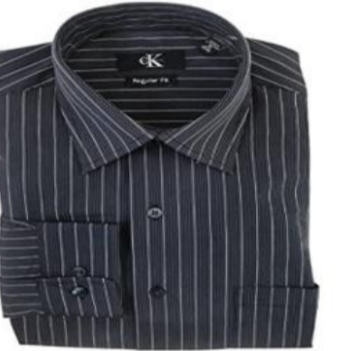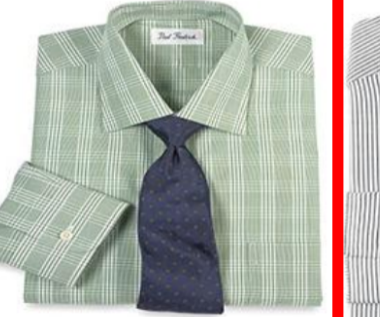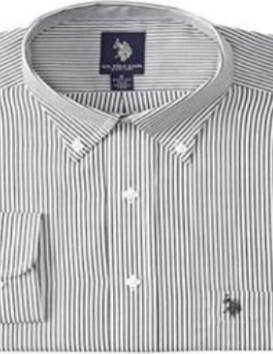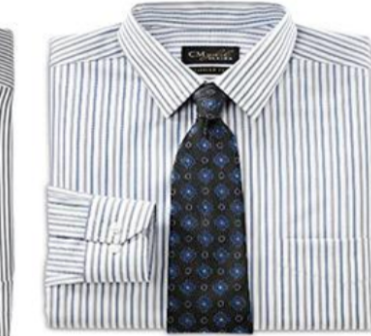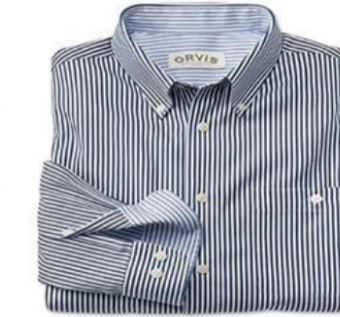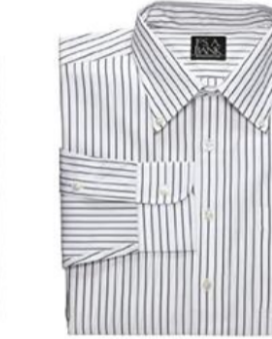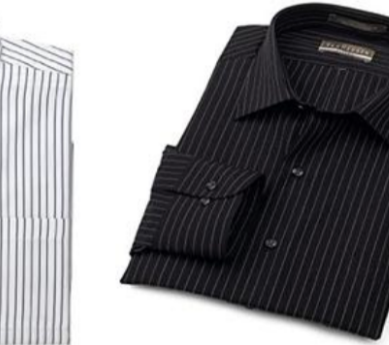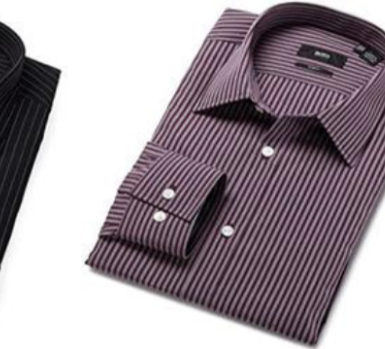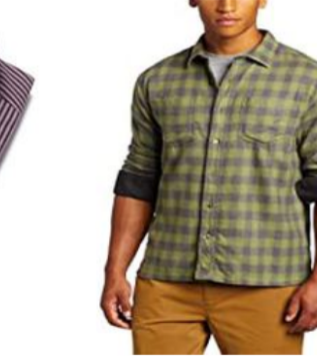

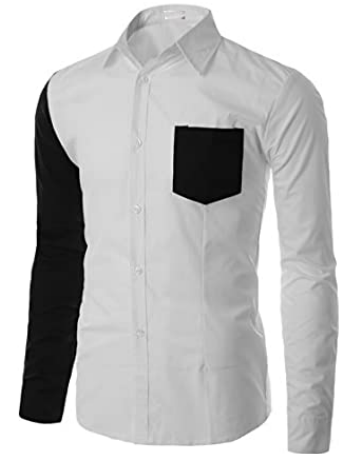

*the shirt is  
white and has  
long sleeves.  
and is lighter  
and more  
western*

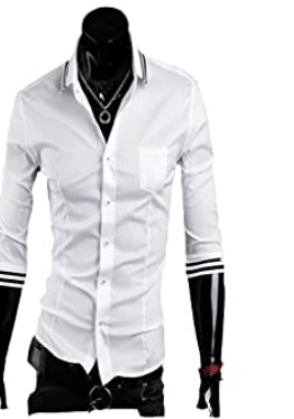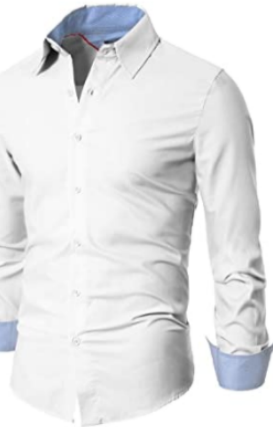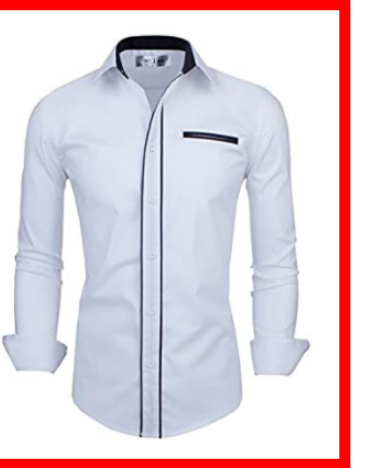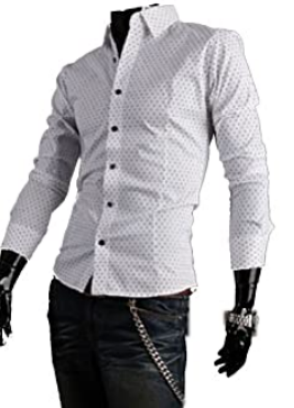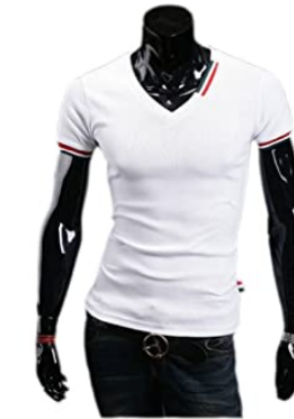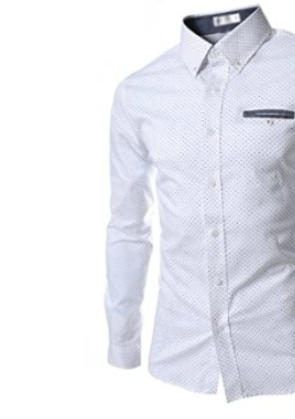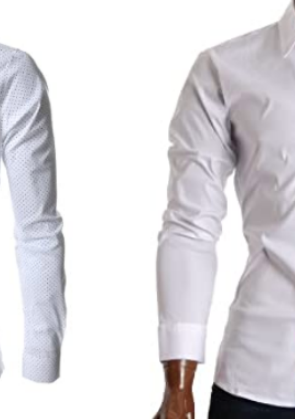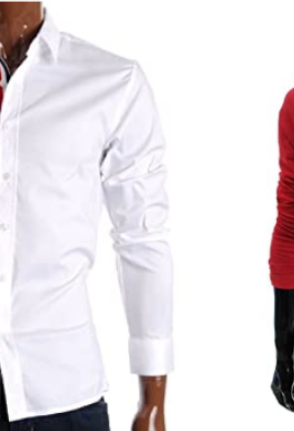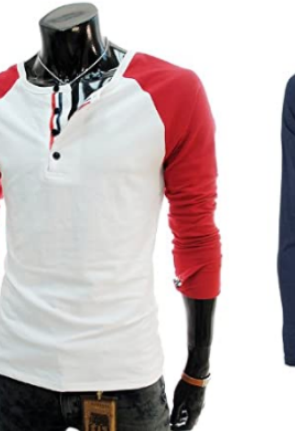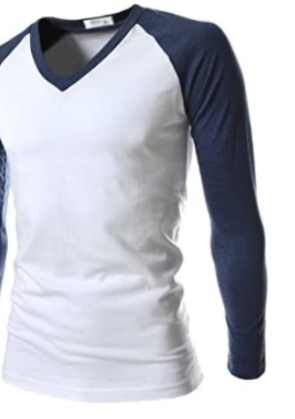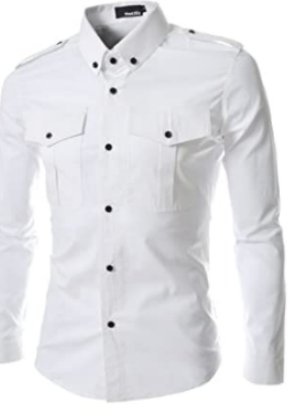

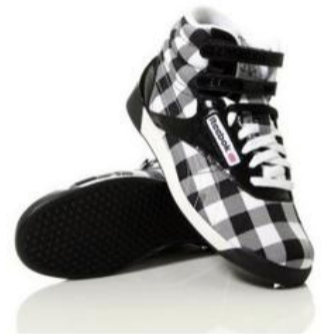

*are more  
solid in black  
with orange-  
and-beige  
trim*

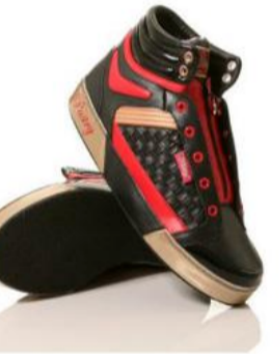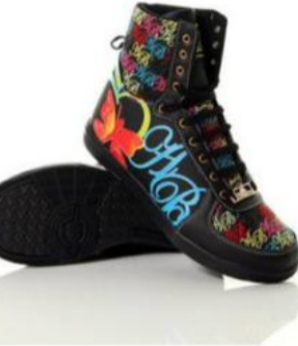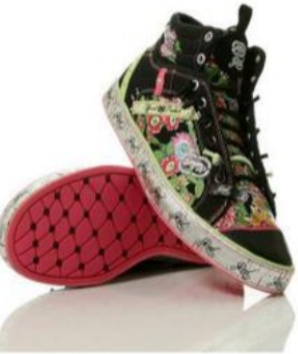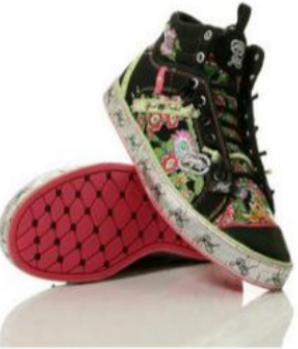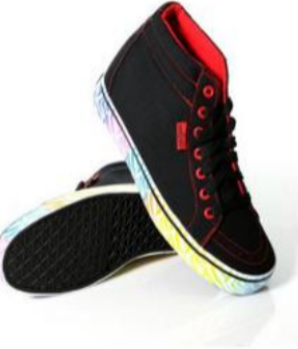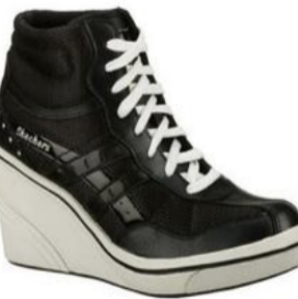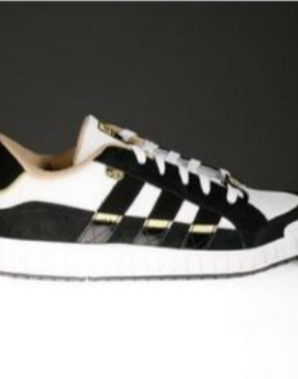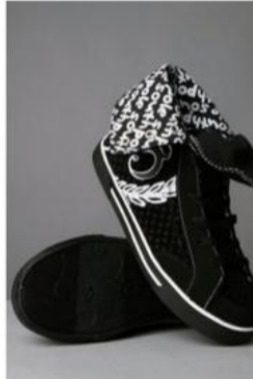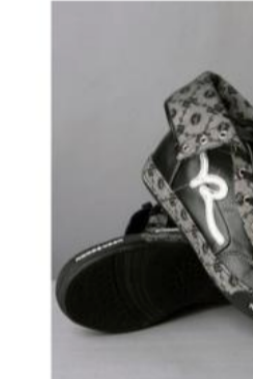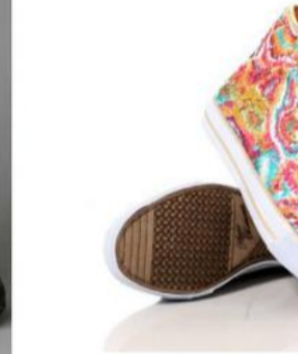

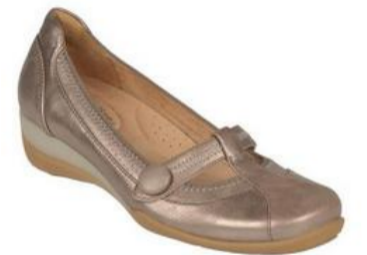

*are tennis  
shoes that  
are black and  
yellow and  
blue*

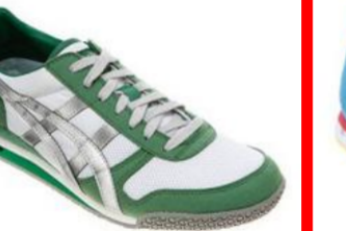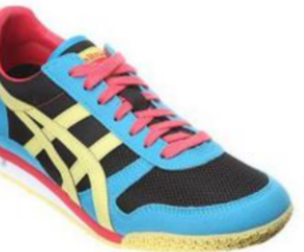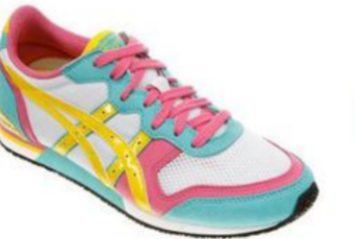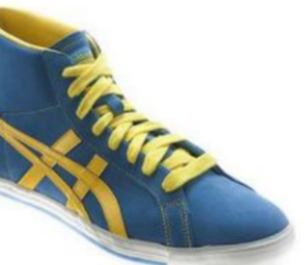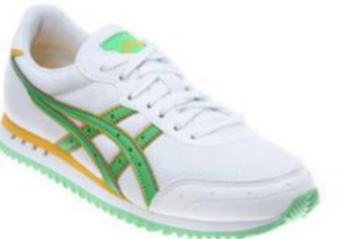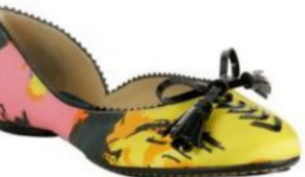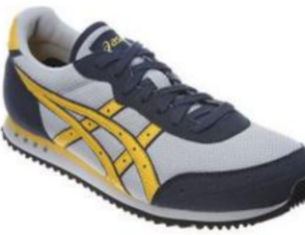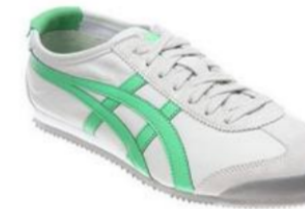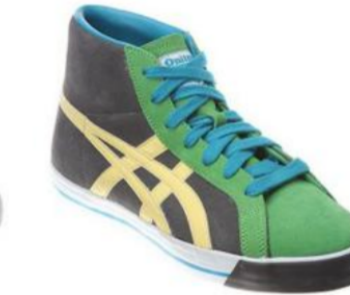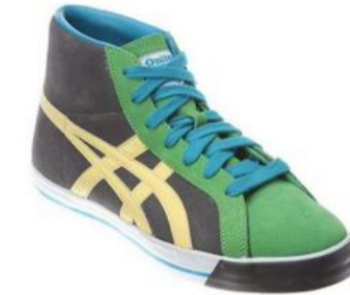

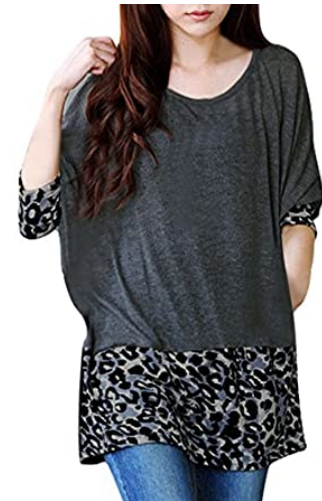

*is yellow  
with fringe  
and is yellow  
with shorter  
sleeves*

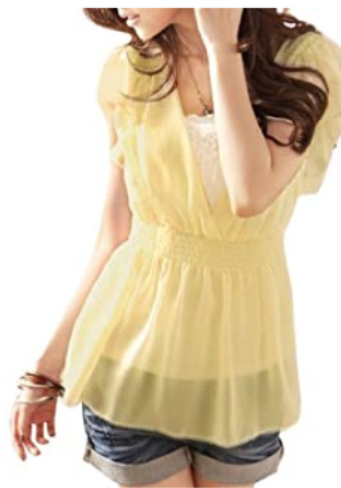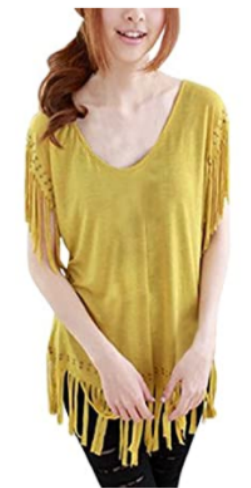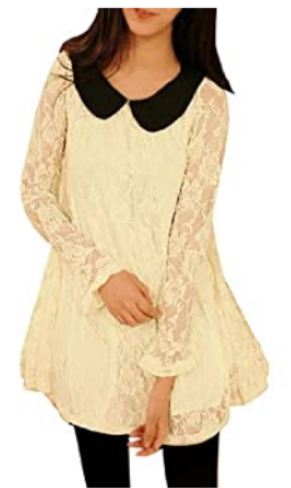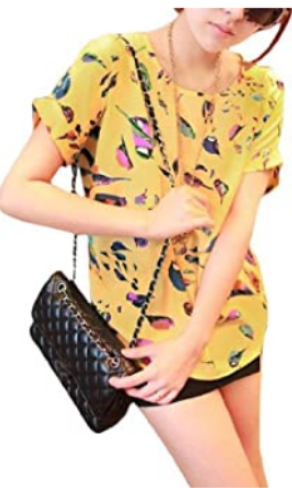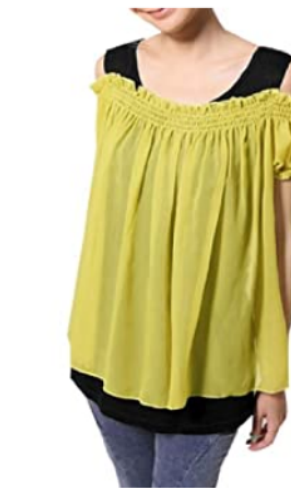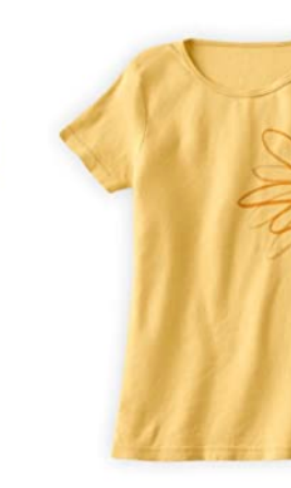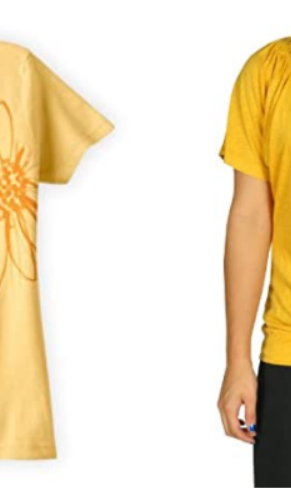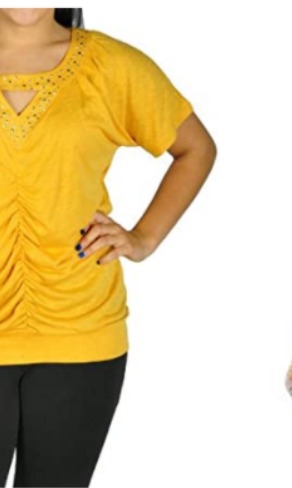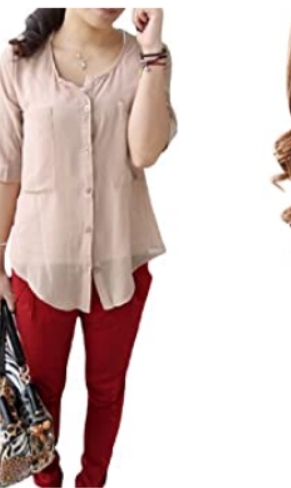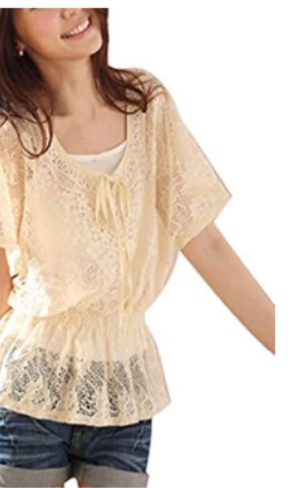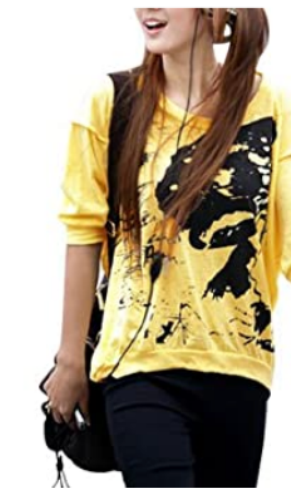

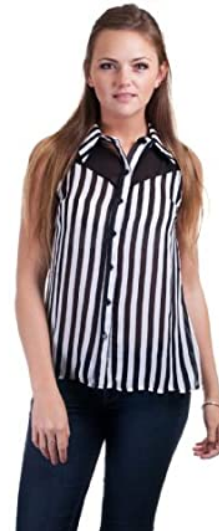

*is white with  
longer sleeves  
and with v  
neckline*

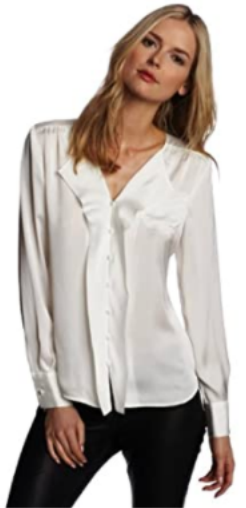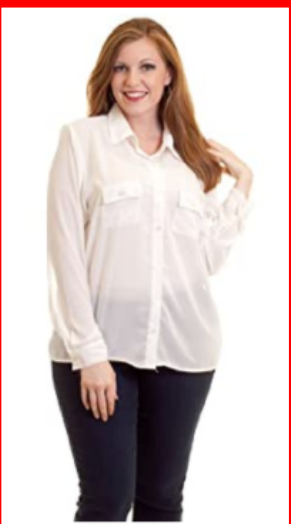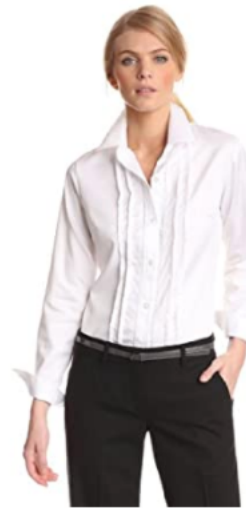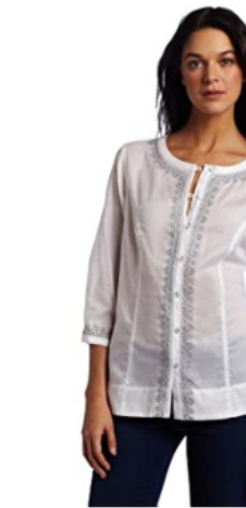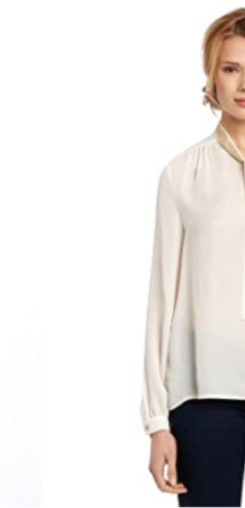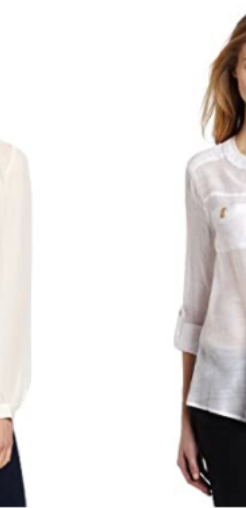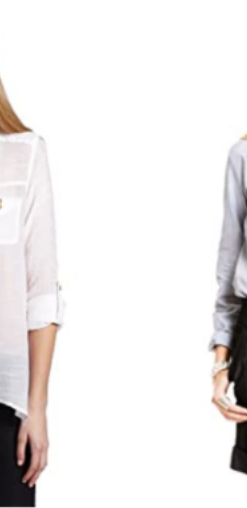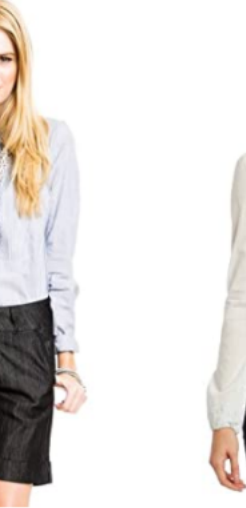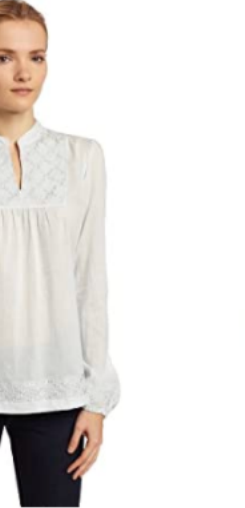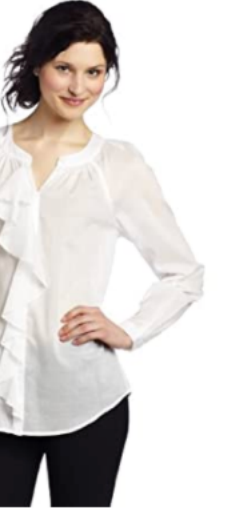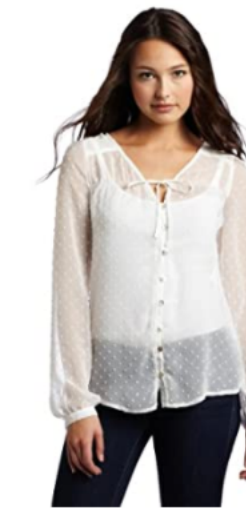

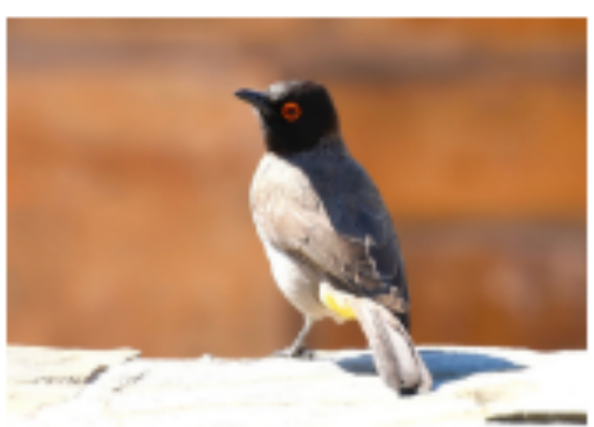

*animal1 has black wings, a black head and beak and a white breast and tail. animal2 has a black breast with green and turquoise flashes. it has a black head and a much longer beak. it has a shorter tail.*

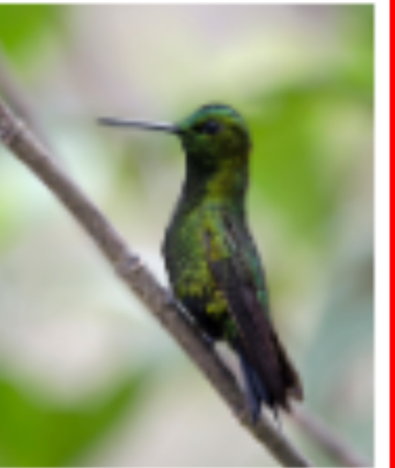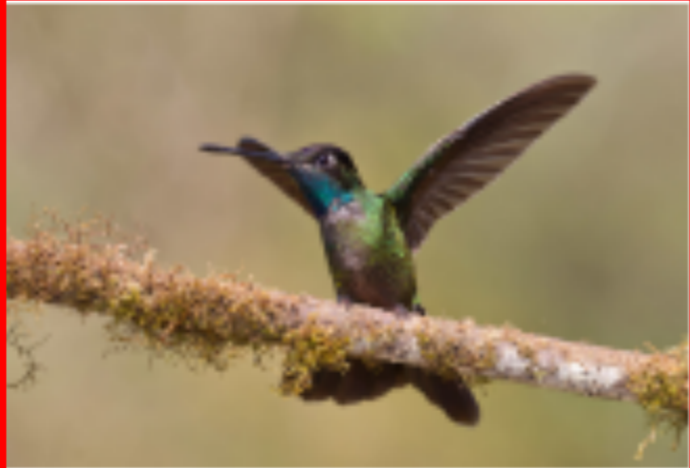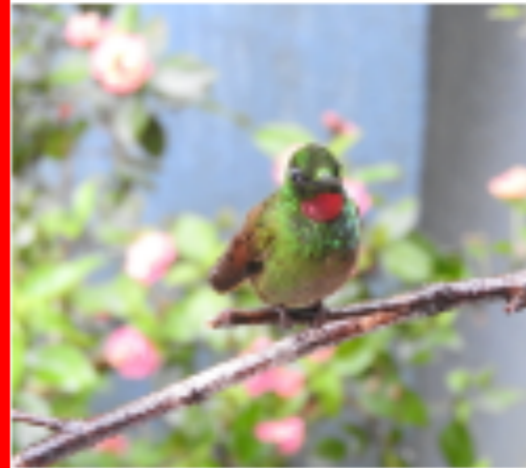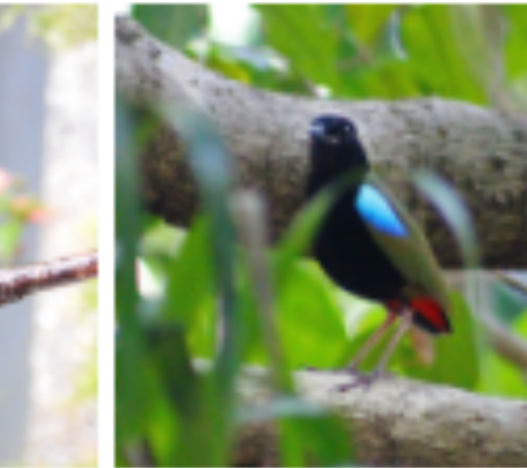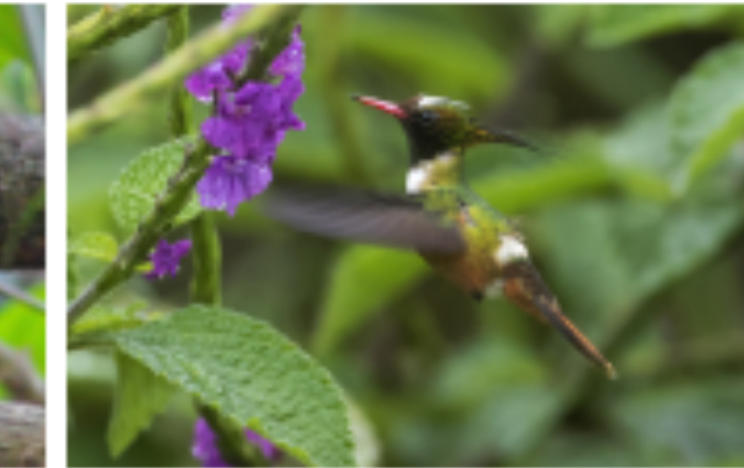

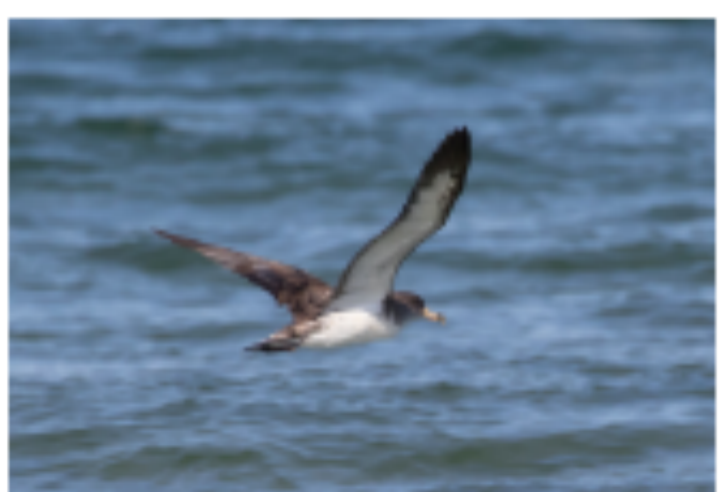

*animal1 is white with  
brown head/wings  
while animal2 is white  
with grey head/wings*

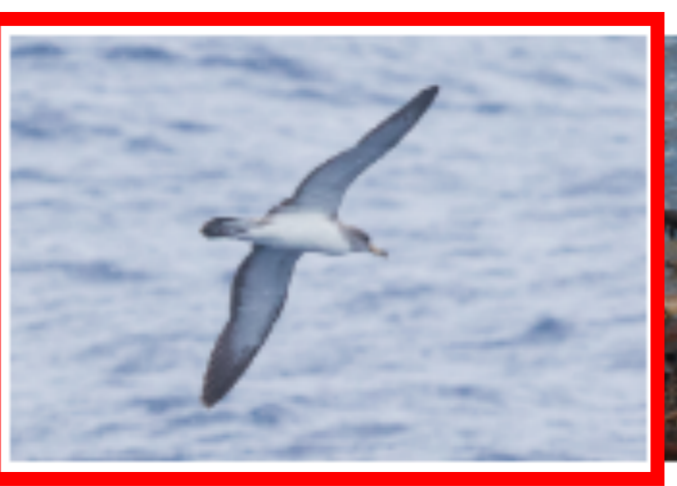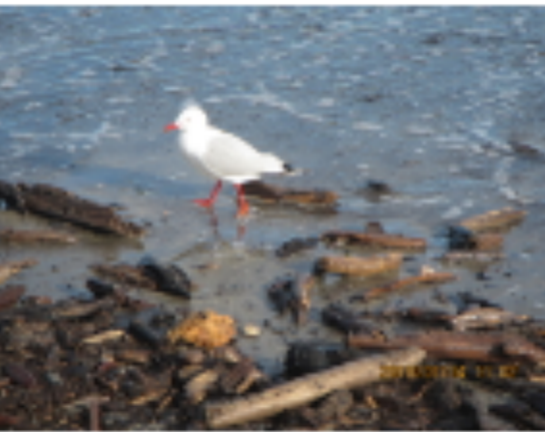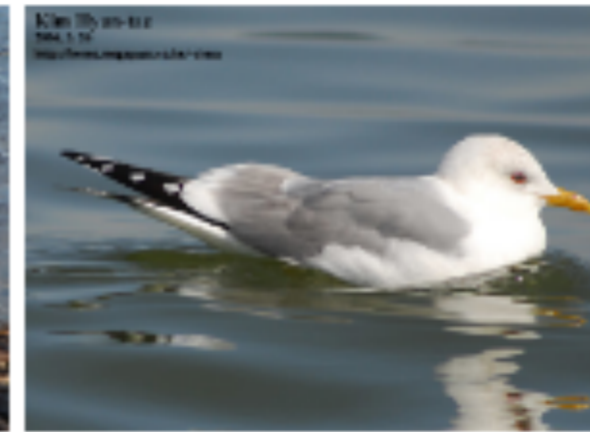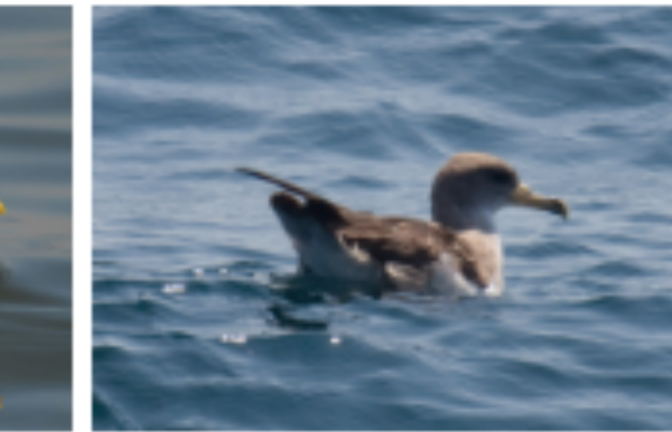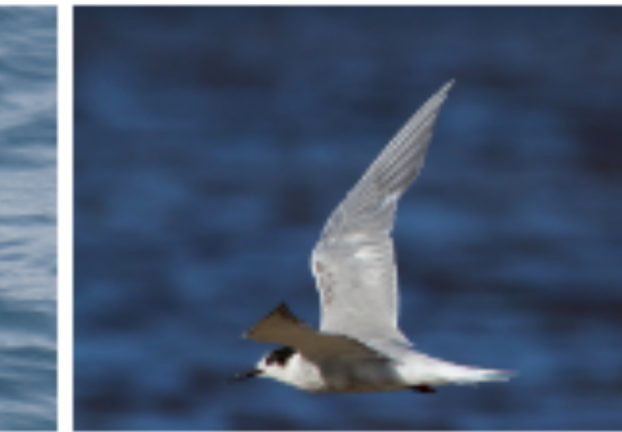

Supplement: Supplementary file 1 [file paper-additional-results.pdf]
